# Supplementary material for: Token-based Vehicular Security System (TVSS): Scalable, Secure, Low-latency Public Key Infrastructure for Connected Vehicles
Source: arXiv:2402.18365 source file (2024-02-28)
Supplement: Supplementary file 1 [file appendix.tex]

\input{crypto_prelim}

\input{security}
